# Supplementary material for: The Four Loop QCD Rapidity Anomalous Dimension
Source: arXiv:2205.02249 ancillary file (2022-07-21)
Supplement: Supplementary file 1 [file ancillary_readme.pdf]

# Ancillary Files for “The Four Loop QCD Rapidity Anomalous Dimension”

Ian Moulton,<sup>1,\*</sup> Hua Xing Zhu,<sup>2,†</sup> and Yu Jiao Zhu<sup>3,‡</sup>

<sup>1</sup>*SLAC National Accelerator Laboratory, Stanford University, CA, 94309, USA*

<sup>2</sup>*Zhejiang Institute of Modern Physics, Department of Physics, Zhejiang University, Hangzhou, 310027, China*

<sup>3</sup>*Bethe Center for Theoretical Physics, Universitat Bonn, D-53115, Germany*

In this note we explain the definitions and conventions for the ancillary files associated with the arXiv submission of “The Four Loop QCD Rapidity Anomalous Dimension”.

| $N_f C_F^3$        | $N_f C_F^2 C_A$      | $N_f d_{FF}^{(4)}/N_c$ | $d_{FA}^{(4)}/N_c$ |
|--------------------|----------------------|------------------------|--------------------|
| $80.780 \pm 0.005$ | $-455.247 \pm 0.005$ | $-143.6 \pm 0.2$       | $-998.0 \pm 0.2$   |

TABLE I: Numerical values for the color coefficients appearing in various anomalous dimensions

## THE FULLY DIFFERENTIAL SOFT FUNCTION AND THE EFFECTIVE COUPLING

In the MATHEMATICA file `fully.m`, we provide expressions for both bare and the  $\alpha_s$ -renormalized fully differential soft functions defined in Eq. (5.3) in the paper, denoted as `FTb` and `FTr` respectively. Note that fully differential soft functions is infrared safe quantity, when expressed by renormalized strong coupling “`as`” =  $\frac{\alpha_s(\mu)}{4\pi}$ , they do not develop any poles in the  $\epsilon$ -expansion. Note that in the expression of `FTb` we use bare coupling “`asb`” =  $\frac{\alpha_s}{4\pi}$  as expansion parameters.

## THE TMD SOFT EXPONENT

In the MATHEMATICA file `SoftExponent.m`, we provide the renormalized TMD soft exponent up to 3-loop, the bare soft exponent are related to the fully differential soft function through integration Eq. (6.1) in the paper. The scale logarithms appeared in the expressions are defined by

$$\text{Lb} = L_b = \ln(|b_\perp^2| \mu^2 / b_0^2), \quad \text{Lr} = L_r = \ln(\nu^2 \vec{b}_\perp^2 / b_0^2), \quad (1)$$

where  $b_0 = 2e^{-\gamma_E}$ . The soft exponent are calculated from irreducible web diagrams, and the normal TMD soft function can be obtained from the soft exponent by non-abelian exponentiation.

## THE ANOMALOUS DIMENSIONS

In the MATHEMATICA file `anomaN4L0.m`, we provide all the relevant anomalous dimensions up to 4-loop, including quark and gluon virtual anomalous dimensions, soft and rapidity anomalous dimensions. Note that quark

and gluon soft and rapidity anomalous dimensions are related by generalized Casimir scaling, we use the following symbols to denote their dependence on the exact representation,

for fundamental representation,

$$N_r = N_c, \quad C_r = C_F, \quad \text{d4FR} = d_{FF}^{(4)}, \quad \text{d4RA} = d_{FA}^{(4)}, \quad (2)$$

and for adjoint representation,

$$N_r = N_a, \quad C_r = C_A, \quad \text{d4FR} = d_{FA}^{(4)}, \quad \text{d4RA} = d_{AA}^{(4)}. \quad (3)$$

In our results there appear four symbols that are known numerically, we list them in Table I according to the work [3]. Except for these four numerical values we arrive at a fully analytical form by combing our calculations with the results of the 4-loop collinear anomalous dimensions [1, 2].

## SYMBOLS AND COLORS

For the color factors in QCD,

$$\begin{aligned} \text{nc} &= N_c = 3, \quad \text{na} = N_a = 8, \\ \text{CF} &= C_F, \quad \text{Nf} = N_f, \quad \text{TF} = T_F, \quad \text{CA} = C_A, \\ \text{d4FF} &= d_{FF}^{(4)} = \frac{(N_c^4 - 6N_c^2 + 18)(N_c^2 - 1)}{96N_c^2}, \\ \text{d4FA} &= \text{d4AF} = d_{FA}^{(4)} = d_{AF}^{(4)} = \frac{N_c(N_c^2 + 6)(N_c^2 - 1)}{48}, \\ \text{d4AA} &= d_{AA}^{(4)} = \frac{N_c^2(N_c^2 + 36)(N_c^2 - 1)}{24}. \end{aligned} \quad (4)$$

`plusD[n,x]` is the conventional plus distribution

$$\text{plusD}[\mathbf{n}, \mathbf{x}] = \left[ \frac{\ln^n(x)}{x} \right]_+. \quad (5)$$

Dirac delta function is represented by

$$\text{plusD}[-1, \mathbf{x}] = \delta(x).$$

Harmonic polylogarithms are represented by

$$\text{H}[\mathbf{a1}, \mathbf{a2}, \dots, \mathbf{an}, \mathbf{x}] = \text{HPL}[\{\mathbf{a1}, \mathbf{a2}, \dots, \mathbf{an}\}, \mathbf{x}],$$

and `zeta[n]` is Riemann zeta value  $\zeta_n$ .

---

\* imoult@slac.stanford.edu

† zhuhx@zju.edu.cn

‡ yzhu@uni-bonn.de

- [1] R. N. Lee, A. von Manteuffel, R. M. Schabinger,  
A. V. Smirnov, V. A. Smirnov and M. Steinhauser,

“Quark and gluon form factors in four-loop QCD,”  
[arXiv:2202.04660 [hep-ph]].

- [2] B. Agarwal, A. von Manteuffel, E. Panzer and R. M. Schabinger, “Four-loop collinear anomalous dimensions in QCD and  $\mathcal{N} = 4$  super Yang-Mills,” [arXiv:2102.09725 [hep-ph]].
- [3] G. Das, S. O. Moch and A. Vogt, “Soft corrections to inclusive deep-inelastic scattering at four loops and beyond,” JHEP **03**, 116 (2020) doi:10.1007/JHEP03(2020)116 [arXiv:1912.12920 [hep-ph]].
